# Supplementary material for: Correlation of tunnel magnetoresistance with the magnetic properties in perpendicular CoFeB-based junctions with exchange bias
Source: arXiv:1802.08002 ancillary file (2018-10-05)
Supplement: Supplementary file 1 [file Supplementary_Material.pdf]

# - Supplementary Material -

# Correlation of tunnel magnetoresistance with the magnetic properties in perpendicular CoFeB-based junctions with exchange bias

Orestis Manos[1], Panagiota Bougiatioti[1], Denis Dyck[1], Torsten Huebner[1], Karsten Rott[1], Jan-Michael Schmalhorst[1] and Günter Reiss[1]
[1] *Center for Spinelectronic Materials and Devices, Department of Physics, Bielefeld University, Universitätsstraße 25, 33615 Bielefeld, Germany*

(Dated: October 5, 2018)

## I. MAGNETIC MEASUREMENTS AT SEVERAL POST ANNEALING TEMPERATURES

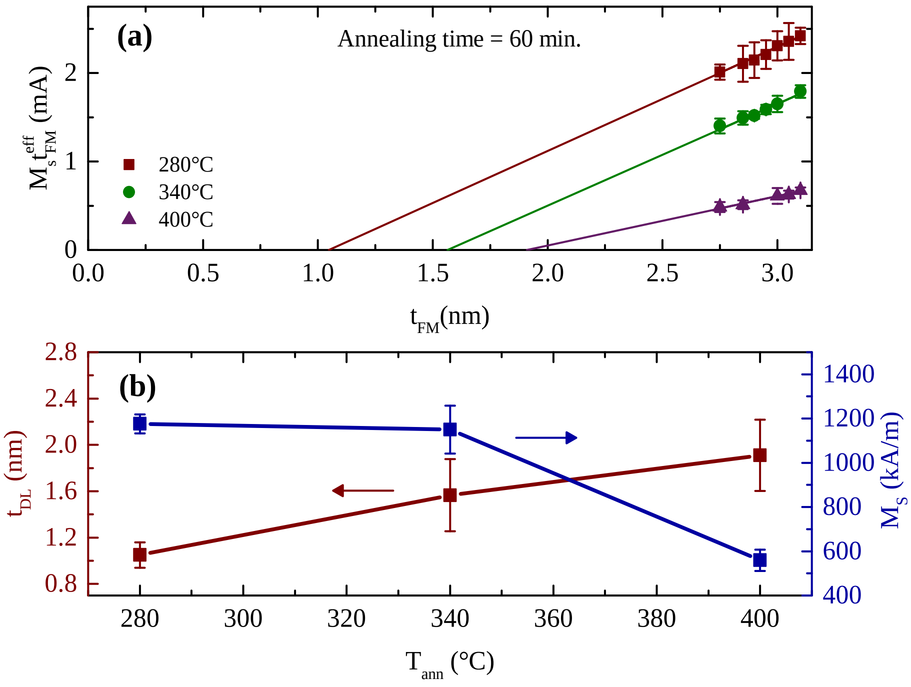


FIG. S 1. (a) Saturation magnetization per unit area $M_s t_{FM}^{eff}$ plotted against the ferromagnetic thickness $t_{FM}$. (b) Magnetic dead layer thickness $t_{DL}$ (left-axis) and saturation magnetization $M_s$ (right-axis) as a function of the annealing temperature $T_{ann}$.

Figure S1(a) illustrates the saturation magnetization per unit area $M_s t_{FM}^{eff}$ as a function of the ferromagnetic thickness with the corresponding linear fit for post-annealing temperatures equal to $T_{ann} = 280, 340, 400\,°C$ for the sample series with $t_{Ta}^{int} = 0.4\,nm$. The dead layer thickness $t_{DL}$ is estimated from the intercept of the linear fit with $M_s t_{FM}^{eff} = 0$. From the slopes of the curves the saturation magnetization $M_s$ is extracted. In Fig. S1(b) the $t_{DL}$ (left-axis) and $M_s$ (right-axis) are presented for $T_{ann} = 280, 340, 400\,°C$. Specifically, the $M_s$ values are found to be equal to $M_s = (1176 \pm 43)\,kA/m$ for $T_{ann} = 280\,°C$, $M_s = (1150 \pm 108)\,kA/m$ for $T_{ann} = 340\,°C$, and $M_s = (559 \pm 48)\,kA/m$ for $T_{ann} = 400\,°C$. Furthermore, the $t_{DL}$ are extracted to be equal to $t_{DL} = (1.05 \pm 0.11)\,nm$ for $T_{ann} = 280\,°C$, $t_{DL} = (1.56 \pm 0.31)\,nm$ for $T_{ann} = 340\,°C$, and $t_{DL} = (1.91 \pm 0.30)\,nm$ for $T_{ann} = 400\,°C$. These results are in line with previous publications [1], where $M_s$ and $t_{DL}$ present similar dependency on $T_{ann}$. Nonetheless, Jang *et al.* [2] reported an increase of $M_s$ with increasing $T_{ann}$ as a consequence of the enhanced crystallization of the CoFeB layer.

In order to interpret the difference of the reported results, one could argue that the parameter $M_s$ is sensitive twofold. On the first hand, it depends on the amount of boron (B) located in the CoFeB electrode and on the other hand

is affected by the $t_{DL}$. The deficiency of B would enhance the crystallization of CoFeB and, thus, the resulting $M_s$. While, the formation of $t_{DL}$ would lead to the decrease of the determined $M_s$. The domination of the one mechanism over the other determines the final result. Consequently, the formation of the dead layer with increasing $T_{ann}$, can obscure the effect of B absorption, resulting in lower $M_s$ values, as Sinha *et al.* [3] have reported in their work.

## II. DEPENDENCE OF HYSTERESIS LOOPS, MAGNETOSTATIC COUPLING AND EB ON THE ANNEALING TIME

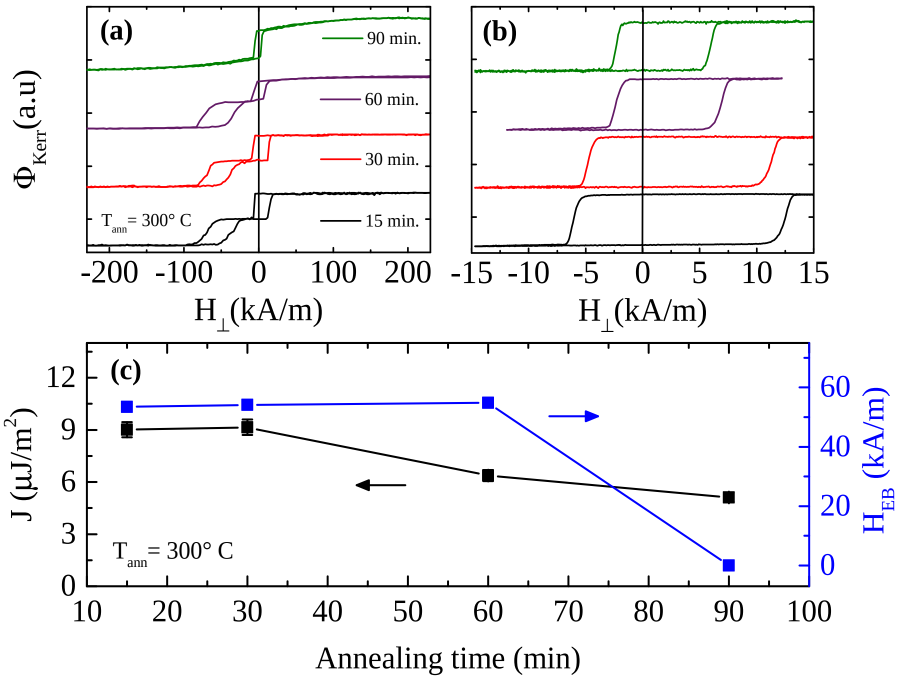


FIG. S 2. (a) Major and (b) minor normalized hysteresis loops of stacks with $t_{MgO} = 2\,nm$, $t_{Ta}^{int} = 0.4\,nm$, and $t_{CoFe+CoFeB} = 3\,nm$, for $T_{ann} = 300\,°C$ and annealing time = 15 (black), 30 (red), 60 (purple), 90 (green) min. (c) The dependence of $J$ (left-axis) and $H_{EB}$ (right-axis) on annealing time for $T_{ann} = 300\,°C$.

Figures 2(a) and (b) show a number of representative normalized major and minor hysteresis loops for $t_{MgO} = 2\,nm$ and $t_{Ta}^{int} = 0.4\,nm$ at $T_{ann} = 300\,°C$ and for several annealing times equal to 15 (black), 30 (red), 60 (purple), 90 (green) min., respectively. Specifically, from Fig. 2(a) the loss of EB in the pinned part can be extracted for the annealing time equal to 90 min. In addition, Fig. 2(b) illustrates the progressive reduction of $H_s$ of the free layer with increasing $T_{ann}$. Figure 2(c) shows the dependence of $J$ (left-axis) and $H_{EB}$ (right-axis), on annealing time extracted from the minor and major loops. As visible, the annealing time causes a progressive degradation of $J$. On the contrary, the $H_{EB}$ presents stable values for the annealing time range (15-60) min. and disappears for annealing time equal to 90 min.

[1] A. Kaidatzis, C. Bran, V. Psycharis, M. Vázquez, J. M. García-Martín, and D. Niarchos, Appl. Phys. Lett. **106**, 262401 (2015).
[2] S. Y. Jang, C.-Y. You, S. H. Lim, and S. R. Lee, J. Appl. Phys. **109**, 013901 (2011).
[3] J. Sinha, M. Gruber, M. Kodzuka, T. Ohkubo, S. Mitani, K. Hono, and M. Hayashi, J. Appl. Phys. **117**, 043913 (2015).
